# Supplementary material for: SkillWrapper: Generative Predicate Invention for Task-level Robot Planning
Source: arXiv:2511.18203 source file (2026-09-28)
Supplement: Supplementary file 1 [file __operator_learning.tex]

\textcolor{red}{
    \textbf{Hypothesis to prove}: for either of the two directions we cannot prove, if it ever happens, i.e., 
}
$$ \color{red} \exists\, \Ground{\operator} \in \Ground{\Operators}_\skill,\ \state_\text{pre} \models \PRE[\Ground{\operator}] \text{ but }  \tau \notin \cD_\skill^{success}, $$
\textcolor{red}{
    or
}
$$ \color{red} \tau \notin \cD_\skill^{success} \text{ but }\exists\, \Ground{\operator} \in \Ground{\Operators}_\skill,\ \state_\text{pre} \models \PRE[\Ground{\operator}], $$
\textcolor{red}{
    it would be the same as case $d$ in the Venn diagram, and can only be solved by predicate invention.
}

Suppose that \sys{} learns a set of operators $\Operators$ using $\cD$.

\begin{lemma}
Let $\Operators_\skill$ be the set of operators learned from a subset of transitions $\cD_\skill \subseteq \cD$, all involving instances of some skill $\skill$. Then, for an observed transition $\tau = \Tuple{\state_\text{pre}, \skillInstance, \state_\text{post}}$, some learned ground operator's preconditions are satisfied by its pre-state $\state_\text{pre}$ if and only if that transition was successful:
$\big( \exists\, \Ground{\operator} \in \Ground{\Operators}_\skill,\ \state_\text{pre} \models \PRE[\Ground{\operator}] \big) \iff \big( \tau \in \cD_\skill^{success} \big)$.
\end{lemma}

\textit{Proof.} For each operator $\operator \in \Operators_\skill$, there exists a subset $\bm{d}_\skill \subseteq \cD_\skill^{success}$ with corresponding abstract effects.\footnote{This is true because each learned operator corresponds to a cluster of abstract effects from successful transitions. If one of those clusters were empty, we wouldn't invent a corresponding operator.}
Also, recall that for a given cluster of lifted effects, \sys{} computes its operator's preconditions as $\PRE = \cap_{\Tuple{\state_\text{pre}^i, \skillInstance^i, \state_\text{post}^i} \in \bm{d}_\skill} \AbstractionF(\state_\text{pre}^i)$.

($\implies$ \textbf{contradicted}) Suppose that the preconditions of one of the learned ground operators are satisfied by the pre-state of some transition in the skill-relevant dataset $\cD_\skill$.
Then we know that there exists a corresponding (non-grounded) operator $\operator$, and a subset of the skill-relevant dataset (say, $\bm{d}_\skill$) corresponding to that operator.
However, because \sys{} learns operators using only the successful transitions, we cannot say anything about the pre-states of \emph{failed} transitions in relation to $\operator$.
Further, because preconditions are computed as intersections over observed examples, the precondition sets will necessarily be minimal, making it more plausible that a failed transition might satisfy one of the operator's preconditions \emph{by coincidence}.
Specifically, when we begin predicate invention and operator learning, the predicate set is empty, and each skill has a single corresponding operator with empty preconditions and effects.
At this point, we would expect \emph{any} transition to satisfy its skill's sole operator's preconditions, contradicting this direction of this lemma. \textcolor{red}{$\not \Box$}

($\impliedby$) Suppose that we have a successful transition in $\cD^{success}_\skill$ involving an instance of the skill $\skill$. Then this successful transition will be used for operator learning and will appear in one of the lifted effects clusters for the skill.
By the definition of how \sys{} learns $\PRE$, the preconditions for the operator corresponding to that cluster are an intersection \emph{including} the abstract pre-state of the successful transition.
The skill instance's arguments fix the objects used to define the relevant ground operator $\Ground{\operator}$.
By the definition of intersection, $\PRE[\Ground{\operator}] \subseteq \alpha(\state_\text{pre})$, which means that the pre-state satisfies the ground operator's preconditions. \qed

\begin{lemma}
Let $\Operators_\skill$ be the set of operators learned from a subset of transitions $\cD_\skill \subseteq \cD$, all involving instances of some skill $\skill$. Given a transition $\tau$ from the skill-relevant dataset $\cD_\skill$, if none of the skill's ground operators $\Ground{\operator} \in \Ground{\Operators}_\skill$ have their preconditions satisfied by the transition's pre-state, then the transition must have failed:
$\big( \not \exists \Ground{\operator} \in \Ground{\Operators}_\skill,\ \state_\text{pre} \models \PRE[\Ground{\operator}] \big) \implies \big( \tau \in \cD_\skill^{fail} \big)$.
\end{lemma}
