# Supplementary material for: SkillWrapper: Generative Predicate Invention for Task-level Robot Planning
Source: arXiv:2511.18203 source file (2026-09-28)
Supplement: Supplementary file 2 [file full_formal_framework.tex]

% In this section, we define our problem setting and the concepts required to understand our method.
%
We consider a problem setting in which a robot is equipped with a set of predefined, ``black-box'' skills.
%
The robot can evaluate whether a skill is executable in the current state, but it does not have a complete transition model of the skills a priori,
%
and therefore cannot compose its skills to solve long-horizon problems without considering low-level details.
%
However, if the agent were to learn symbolic models of its skills, it could use classical planning to efficiently compose them to solve new tasks.
%
%This        We - Kept for comment
%
In this section, we formalize this setting as the problem of \emph{Skill Model Learning}.
%, and define the concepts required to understand our method.
% learning \emph{Skill Abstraction}s.
%
% We then define formal properties that any method for active skill abstraction might aim to achieve.

\subsection{Preliminaries}

\paragraph{Environment Model.}{
    % As the agent learns to compose its skills across a range of settings, the agent itself and its skills remain the same.
    % %
    % Consequently, our model differentiates between aspects of the problem that remain the same---the \emph{environment}---and those that vary between different \emph{settings}.
    % %
    %Formally, 
    We define an \emph{environment} as a tuple $\DefDomain$, where the \emph{state space} $\States$ is assumed to be high-dimensional, continuous, and fully observable; %(i.e., each state $s \in \mathbb{R}^n$).
    %
    the \emph{type set} $\Types$ enumerates the possible object types;
    %
    and the \emph{skills} $\Skills$ are object-centric, such that each $\skill \in \Skills$ is parameterized by object types drawn from the \emph{type set} $\Types$.
    %
    The \emph{transition function} $\DefTransitionFunction$ characterizes the environment dynamics but is unknown to the agent.
% The agent is equipped with \emph{object-centric skills} $\skill \in \Skills$ parameterized by object types drawn from the \emph{type set} $\Types$.
    % %
    % The agent is equipped with \emph{object-centric skills} $\skill \in \Skills$ parameterized by object types drawn from the \emph{type set} $\Types$.
    %
    For example, \texttt{Pour(?teapot,}~\texttt{?mug)} may be used to pour tea from a teapot into a mug.
    %
    However, certain environmental aspects (e.g., which mugs are available to pour into) may differ between settings during learning.
    %
    We therefore define a specific \emph{setting} by the tuple $\DefSetting$, specifying an initial state $\initialState \in \States$ and a set of typed objects $\Objects$, where the type(s) of object $\object \in \Objects$ are denoted by $\typeOf{\object} \subseteq \Types$.
    %
    % shared across all environments... (on the set of skills)
}\label{sec:environment-model}

\paragraph{Black-box Skills.}{
    We model skills as object-centric options~\citep{sutton1999options} with discrete, object-typed parameters.
    %
    Formally, a \emph{skill} $\skill \in \Skills$ is defined by a tuple $\DefSkill$,
    %
    where the \emph{initiation set} $\InitiationSetOf{\skill} \subseteq \States$ contains states from which the skill may be executed;
    %
    the \emph{policy}~$\OptionPolicy$ controls the agent during the skill;
    %
    the \emph{termination set} $\TerminationSet \subseteq \States$ is the set of states at which the skill immediately terminates;
    %
    and the \emph{skill parameters} $\DefParametersOf{\skill}{k}$ specify type constraints $\typeOf{\parameterOf{\skill}^i} \subseteq \Types$ for valid skill arguments.
    %
    Specifically, a skill $\skill \in \Skills$ may be instantiated to create a \emph{skill instance} $\skillInstance$ using objects $\NTupleOf{k}{\object} \in \Objects^k$ if and only if for $1 \leq i \leq k$, $\typeOf{\parameterOf{\skill}^i} \subseteq \typeOf{\object_i}$.
    %
    We assume that executing a skill only affects the state of objects passed as arguments.\footnote{We do not, however, assume that a skill necessarily affects the state of \emph{all} objects passed in as arguments.}
}

\paragraph{Symbolic Abstractions.}
% \textcolor{red}{did we say we only consider less than 2-arity predicates?}
%
Because the agent must evaluate $\InitiationSetOf{\skill}$ on individual states, it cannot distinguish essential skill information from irrelevant details, making long-horizon planning combinatorially difficult.
%
%, as each state is treated as a separate atomic entity.
%
However, each skill affects only a few objects at once, leaving the rest of the world unchanged.
%
The agent can exploit this property by instead learning a factored state representation---formalized here as first-order logic models in PDDL~\citep{mcdermott1998pddl}---providing an abstract transition model of its skills.
%
Such abstractions enable the agent to use classical planning to compose its skills and accomplish unseen, long-horizon goals.


We use symbolic \emph{predicates} $\Predicates$ to express abstract relations between objects.
%
Each predicate $\predicate \in \Predicates$ is a tuple $\DefPredicate$, where the \emph{predicate classifier} $\PredicateClassifier$ tests whether the predicate holds in a state, given a binding of objects to the \emph{predicate parameters} $\DefParametersOf{\predicate}{n}$.
%
Each parameter $\parameterOf{\predicate}^i$ specifies a type constraint $\typeOf{\parameterOf{\predicate}^i} \subseteq \Types$ on corresponding object arguments.
%
Formally, the partial function
% \footnote{We denote a partial function using $f:\mathcal{X} \rightharpoonup \mathcal{Y}$.}
%
\mbox{$\DefPredicateClassifier$} is defined on objects $\NTupleOf{n}{\object} \in \Objects^n$ if and only if $\typeOf{\parameterOf{\predicate}^i} \subseteq \typeOf{\object_i}$ for $1 \leq i \leq n$.
%
In such cases, we say that the objects $\NTupleOf{n}{\object}$ are \emph{valid arguments} for $\predicate$.

%
% Comment
%

% Using the invented predicates $\Predicates$, the learning method must construct a set of \textit{operators} (i.e., relational abstract actions) defining abstract transition models for the agent's skills. 
By observing different effects, the agent must construct a set of \textit{operators} $\Operators$ that define abstract transition models for the agent's skills.
%
% These transition models are represented using the set of predicates $\Predicates$.
%
We define each operator $\operator \in \Operators$ by $\DefOperator$, 
%
where $\operatorSkill \in \Skills$ is the corresponding skill;
%
the \emph{operator parameters} $\DefParametersOf{\operator}{m}$ impose type constraints $\typeOf{\parameterOf{\operator}^i} \subseteq \Types$ on operator arguments;
%
the \emph{preconditions} $\PRE$ are a conjunction of literals over $\Predicates$ defining the conditions necessary to apply the operator;
%
and the \emph{add} and \emph{delete effects}, $\AddEFF$ and $\DeleteEFF$, are the subsets of $\Predicates$ that become true and false, respectively, after the operator is applied.

\paragraph{Grounded Abstractions.} To apply an abstract transition model to a real-world setting, the agent must map the low-level state to an abstract state, which requires \emph{grounding} the known predicates using concrete objects so that their truth value may be determined.
%
% To apply the abstract transition model to a real-world setting, an agent needs to appropriately map the state of the real world to an abstract state, which requires determining the truth value of known predicates.
%
A predicate $\predicate \in \Predicates$ may only be grounded using valid arguments, inducing a \emph{grounded predicate} $\DefGroundedPredicate$.
%
Given a low-level state, the classifier \mbox{$\DefGroundedPredicateClassifier$} tests whether the predicate holds for the object arguments.
%
% We can evaluate whether a predicate $\predicate \in \Predicates$ holds for specific objects $\object_{1:n} \in \Objects$ in a state $\state \in \States$ by first \emph{grounding} the predicate by binding the objects comprising that state to the predicate parameters $\ParametersOf{\predicate}$.
%
We define the set of \emph{grounded predicates} for a setting $\DefSetting$ under predicates $\Predicates$ as \mbox{$\DefGroundedPredicates$}, inducing an \emph{abstract state space} $\DefAbstractStates$ where each abstract state corresponds to a specific combination of grounded relations.

% The \emph{abstraction function} $\DefAbstractionFunction$ formalizes this relationship by mapping each low-level state $\state \in \States$ to an abstract state $\abstractState \in \AbstractStates$ corresponding to the subset of grounded predicates true in the state.

% \begin{equation}
%     \abstractState = \AbstractionFunction(\state) \triangleq \{ \groundedPredicate \; | \; \groundedPredicate \in \GroundedPredicates \land \GroundedPredicateClassifier(\state) = 1 \}.
% \end{equation}

% David had suggested adding:  where each abstract action corresponds to a black-box skill,

Given a set of operators $\Operators$ in a setting $\DefSetting$, the \emph{abstract action space} $\AbstractActions$ is the set of all valid groundings of the operators using objects from $\Objects$.
%
% The \emph{abstract action space} $\AbstractActions$ is similarly defined by grounding each operator $\operator \in \Operators$ using all valid combinations of objects in the environment.
%
Each \emph{abstract action} (i.e., grounded operator) is defined as $\DefAbstractAction$, where $\operator \in \Operators$, $\NTupleOf{m}{\object} \in \Objects^m$, and for $1 \leq i \leq m$, $\typeOf{\parameterOf{\operator}^i} \subseteq \typeOf{\object_i}$.
%
Grounding an operator induces \emph{ground preconditions} $\GroundPRE$, which are a conjunction of ground literals over $\GroundedPredicates$;
\emph{ground add effects} $\GroundAddEFF \subseteq \GroundedPredicates$;
and \emph{ground delete effects} $\GroundDeleteEFF \subseteq \GroundedPredicates$.

%To express relationships between symbolic abstractions and low-level states
The \emph{grounding function} $\Grounding: \GroundedPredicates \to 2^\States$ maps each grounded predicate to its \emph{grounding set} $\GroundingSetOf{\groundedPredicate} \subseteq \States$, defined as \mbox{$\DefGroundingSet$}.
%
% the set of states in which the grounded predicate is true.
%
We overload this notation for abstract states $\abstractState \in \AbstractStates$ so that \mbox{$\GroundingSetOf{\abstractState} \Def \bigcap_{\groundedPredicate_i \in \abstractState} \GroundingSetOf{\groundedPredicate_i}$}.
%
Conversely, the \emph{abstraction function} $\DefAbstractionFunction$ maps each low-level state $\state \in \States$ to the abstract state $\abstractState \in \AbstractStates$ defined by \mbox{$\AbstractionFunction(\state) \Def \Set{\groundedPredicate \in \GroundedPredicates \SetSuchThat \GroundedPredicateClassifier(\state) = 1}$}.

% An \emph{abstraction function} $\DefAbstractionFunction$ maps each low-level state $\state \in \States$ to an abstract state $\abstractState \in \AbstractStates$ corresponding to the subset of grounded predicates true in the state:

% \begin{equation}
%     \abstractState = \AbstractionFunction(\state) \triangleq \{ \groundedPredicate \; | \; \groundedPredicate \in \GroundedPredicates \land \GroundedPredicateClassifier(\state) = 1 \}.
% \end{equation}

% the \emph{grounding} of an abstract state is the set of low-level states in which all grounded predicates in the abstract state hold.
%
%Finally, the grounding of a set of grounded predicates is the set of low-level states in which all grounded predicates in the set are true.

% $\GroundingSet{\abstractState} = \{ s \in \States \,:\, \forall \groundedPredicate \in \abstractState, \groundedPredicate(s) = 1 \}$

% \textcolor{red}{(Might not be useful anymore since we don't talk about disjunctiveness)In our setting, we assume to have access to a predicate generator $\mathbf{G}$ that proposes predicates $\mathcal{P}$ conditioned on $X \in \mathcal{S}$, such that $\mathcal{G}(\hat{P}) = X$.}

% \subsection{Active Skill Abstraction}
% One aspect that distinguishes our method from Nishanth's papers is the active learning paradigm...

\subsection{Problem Definition}
\begin{definition}
Given an environment $\DefDomain$ containing settings $\{ \DefSetting \}_{i=1}^N$, we define a \emph{Skill Model Learning} problem as learning an \emph{abstract transition model} $\DefModel$ for the skills $\Skills$.
\end{definition}

After a period of continual learning in one or more settings, an agent may be evaluated on an \emph{skill planning problem} $\DefPlanningProblem$, where $\DefGoalStates$ is the set of \emph{goal states} to be reached. 
%
Given a model $\DefModel$, a classical planner can be used to search for an \emph{abstract plan} $\DefAbstractPlan$ that solves the \emph{abstract planning problem} $\DefAbstractPlanningProblem$.
%
\begin{definition}
    An abstract plan $\DefAbstractPlan$ is called a \emph{solution} for skill planning problem \mbox{$\DefPlanningProblem$} iff %, letting $\skillInstance_i$ denote $\skillInstance_{\abstractAction_i}$,
    %
    for $1 \leq i \leq n,\, \state_{i} = \TransitionFunction(\state_{i-1}, \skillInstance_i),
    \state_{i-1} \in \InitiationSetOf{\skillInstance_i},
    \text{ and } \state_n \in \GoalStates,$
    where $\skillInstance_i = \skillInstance_{\abstractAction_i}$.
\end{definition}

% A \emph{solution} to the problem takes the form of a sequence of grounded operators that can map to a \emph{skill plan} (i.e., sequence of skill instances) $\DefPlan$ that reaches a goal state $s_n \in \GoalStates$ from the environment's initial state $\initialState \in \States$.

% \begin{definition}
%     Given an abstract transition model $\mathcal{M}=(\mathcal{P}, \mathcal{A})$ and a skill planning problem $\mathbf{p}$, an \emph{abstract planning problem} requires identifying an abstract plan $[\underline{a}_0, \dots, \underline{a}_{n-1}]$, where $a_i \in \mathcal{A}$, such that the corresponding skill plan $[\skillInstance_0, \dots, \skillInstance_{n-1}]$ is a solution to $\mathbf{p}$.
% \end{definition}

In Sec.~\ref{sec:skillwrapper}, we describe how {\sys} constructs $\gM$ from raw skill executions.
